# Supplementary material for: A Generalized Framework for Video Instance Segmentation
Source: arXiv:2211.08834 source file (2023-03-24)
Supplement: Supplementary file 1 [file supplementary.tex]

\appendix

% --- PDF will be split by an editor (e.g. macOS preview), so need to restart from page 1
%\setcounter{page}{1}

% --- repeat the title (AT: haven't found a more elegant way to do this...)
\twocolumn[
\centering
\Large
\textbf{A Generalized Framework for Video Instance Segmentation} \\
\vspace{3mm}Appendix \\
\vspace{6mm}
] %< twocolumn
%\appendix

\section{Additional Implementation Details}
\label{supp:implementation}

\subsection{Training}
\label{supp:training}
Freezing the frame-level detector~\cite{Mask2Former} during training, we adopt pretrained weight from VITA~\cite{VITA} and finetune the video-level modules only; Object Encoder ($\mathcal{E}$) and Object Decoder ($\mathcal{D}$).
Therefore, our total loss function is same as $\mathcal{L}_{v}$ describe in VITA and we employ same hyper-parameters.
Concretely, 
\begin{equation}
\begin{gathered}
    \mathcal{L}_{v}\text{~\cite{VITA}} = \underbrace{\lambda_{cls}\mathcal{L}_{cls}^{v}}_{\text{categorical loss}} + \underbrace{\lambda_{ce}\mathcal{L}_{ce}^{v} + \lambda_{dice}\mathcal{L}_{dice}^{v}}_{\text{mask-related loss}},\\
\end{gathered}
\end{equation}
where the categorical loss is Cross Entropy and the mask-related loss consists of Binary Cross Entropy loss and Dice loss.
The optimizer is AdamW, and we set the base learning rate and weight decay as 5e-5 and 5e-2 respectively, for all datasets. 
For YouTube-VIS 2019, we train for 15K iters and apply lr decay at 10K iters. 
For YouTube-VIS 2021/2022, we train for 90K iters and apply lr decay at 50K iters. 
And for OVIS, we train for 140K iters and apply lr decay at 100K iters.

\subsection{Inference}
\label{supp:inference}
We use the same inference procedure for all benchmarks and, once again, do not involve any heuristics.
To further specify the inference procedure, we provide simplified PyTorch-style pseudo-codes of our GenVIS in~\cref{alg:genvis}.
Given an input video, we sequentially process non-overlapping clips with predefined length $N_f$.
For each clip, we obtain frame queries (\texttt{fq}) and mask features (\texttt{mf}) from Mask2Former~\cite{Mask2Former} model by feeding backbone features.
Then, the frame queries for the entire clip become the input of Object Encoder.
After that, we generate clip-level predictions through Object Decoder by propagating instance queries (\texttt{q}) from previous clip with stacked memory (\texttt{memory}).
Before going through the following clip, we add encoded instance prototypes (\texttt{p}) of the current clip to the memory.

\section{More Experimental Details}
\label{supp:experimantal_detail}
We provide more experimental details about \cref{tab:ablation_method} in \cref{sec:ablation}.
For the matching algorithm of MinVIS~\cite{MinVIS} used in the baseline, we use the provided code from its official repository.
Since there is no publicly available code for the \textbf{CL} (Correspondence Learning~\cite{EfficientVIS}), we reproduce the algorithm following the description from the original paper~\cite{EfficientVIS}.
We apply the original target assignment algorithm of VITA on the first clip and keep the matched indices on the following clips.
At the inference stage, we do not use heuristics of re-initialization of propagating queries for a fair comparison.

\begin{table}%[H]
	\centering
% 	\begin{minipage}[t]{0.49\linewidth}
%     \caption{
%     %
%     PyTorch-style inference pseudo-code of VITA~\cite{VITA}.
%     % 
%     }
%     \label{alg:vita}
%     \begin{python}
% def vita(video):

%     feats = backbone(video)
%     fq, mf = mask2former(feats)

%     del feats
    
%     fq = object_encoder(fq)
    
%     vq = object_decoder(fq)

%     w = mask_head(vq)

%     # w.shape: (Nv x C)
%     # mf.shape: (C x H x W)
%     pred_mask = w @ mf

%     # Nv x (K+1)
%     pred_cls = cls_head(vq)

%     # Nv x T x H x W
%     pred_mask = torch.stack(
%         pred_mask, dim=1
%     )

%     return pred_cls, pred_mask
%     \end{python}
%     %\vspace{-9mm}
% 	\end{minipage}
% 	\hfill
	% \begin{minipage}[t]{0.49\linewidth}
    
    \begin{python}
def GenVIS(video):
    pred_cls, pred_mask, memory = [], [], []
    q = object_decoder.q
    
    for clip in video:
        feats  = backbone(clip)
        fq, mf = mask2former(feats)
    
        fq     = object_encoder(fq)
        q, p   = object_decoder(fq, q, memory)
        
        memory.append(p)
    
        w = mask_head(q)
        
        # w.shape: (Nq x C)
        # mf.shape: (Nf x C x H x W)
        pred_mask.append(w @ mf)
        pred_cls.append(cls_head(q))
        
    return pred_cls, pred_mask
    \end{python}
    \vspace{-4mm}
	% \end{minipage}
    \caption{
    PyTorch-style inference pseudo-code of GenVIS.
    % \texttt{mf} denotes mask feature of Mask2Former.
    % The arguments of \texttt{object_decoder} are,
    % % 
    }
    \vspace{-5mm}
    \label{alg:genvis}
\end{table}

\section{Additional Qualitative Results}
\label{supp:qualitative}
In \cref{fig:qualitative_supp}, we provide additional qualitative comparisons with state-of-the-art methods that provide checkpoints in official repositories.
%\footnote{We could not include the visualizations of IDOL~\cite{IDOL} because the code provided by its official repository has technical issues to process OVIS dataset.}.
In addition to the results presented in \cref{sec:qualitative}, our method successfully captures highly occluded objects in long sequences.

\section{Dependence on a large amount of labels}
\label{supp:labels}
Designed from a frame-independent detector~\cite{Mask2Former}, MinVIS~\cite{MinVIS} has a great video-data efficiency.
Despite using only 10$\%$ of the data, it still performs competitively, with $-2.2$ AP decrease compared to using all labels on OVIS~\cite{OVIS}.
On the contrary, the effectiveness of GenVIS is largely from its ability to model sequential characteristics of videos from consecutive clips.
Thus, GenVIS does require more video-wise labels than MinVIS.
Following the experimental settings of MinVIS, we trained GenVIS using only 10$\%$ of labels on OVIS with Swin-L.
As can be expected, the reduction of video-wise labels hinders the temporal understanding: it results in drop of $-9.7$ AP ($45.2 \rightarrow 35.5$) compared to full labels.
Our understanding is that GenVIS, which necessitates consecutive frames, faces challenges in learning diverse appearances compared to MinVIS, which uniformly samples frames, despite having the same limited number of frames.

\section{Online inference speed}
\label{supp:labels}
In~\cref{fig:window_size_eval}, we analyze the trade-offs between performance and speed in online \& semi-online setups.
Thanks to its generalized property, GenVIS provides multiple options where users can consider either complexity of datasets or targeted runtime.
Among the varying number of clip lengths, GenVIS shows 18.7 fps on the OVIS benchmark under the online setting ($N_f^{\emph{eval}} = 1$).
We measured the inference speeds of MinVIS~\cite{MinVIS} and IDOL~\cite{IDOL} under a fair evaluation environment, and each achieves 28.1 and 2.1\footnote{IDOL shows the slow inference speed due to its increasing computations with respect to the number of frames for post-processing.} fps, respectively.

\section{Discussions}
\paragraph{Accuracy with the increased number of frames.}
Current offline VIS methods~\cite{Mask2Former-VIS, VITA, SeqFormer} have difficulties in modeling sequential and temporal characteristics of long videos.
Therefore, as GenVIS uses such methods for predictions within a window, the longer window brings about \textit{inaccurate intra-clip predictions} for videos with complicated trajectories, leading to the performance drop ($-12.4$ AP) on the challenging OVIS benchmark (see~\cref{fig:window_size_eval} (b)).
On the contrary, there is a marginal performance drop ($-1.4$ AP) when using longer windows on YouTube-VIS 2019, which comprises relatively simple trajectories.
From the experiments, we would like to highlight our motivation that designing multiple inter-clip associations in a sequential manner is effective rather than simply enlarging a intra-clip window to handle challenging videos.
\paragraph{Accuracy gap between online and semi-online.}
\label{supp:gap}
Intuitively, as discussed in the above paragraph, semi-online methods with an adequate window size have more potentials to achieve higher accuracy than online models.
However, compared to the semi-online versions of GenVIS, the online version can also achieve competitive accuracy as it stores more memories during evaluation.
Affected by these characteristics, the optimal accuracy of GenVIS can be obtained in different settings as each backbone and dataset have different aspects.
An interesting future direction would be to further enhance the intra-clip modeling, which would boost the performance of semi-online VIS, coupled with GenVIS.

% \section{Code}
% \label{supp:code}
% We include the source code to the zip file named \texttt{supp_3917_code.zip}.
% Further implementation details of GenVIS can be found in \texttt{genvis.py}, and the training and inference functions are included in \texttt{meta_arch.py}. 
% In addition, the proposed criterion can be found in \texttt{genvis_matcher.py} and \texttt{genvis_criterion.py}.
% All codes and environmental guidelines for training \& inference will be made publicly available, including trained checkpoints.

\begin{figure*}[t]
\begin{center}
\includegraphics[width=\linewidth]{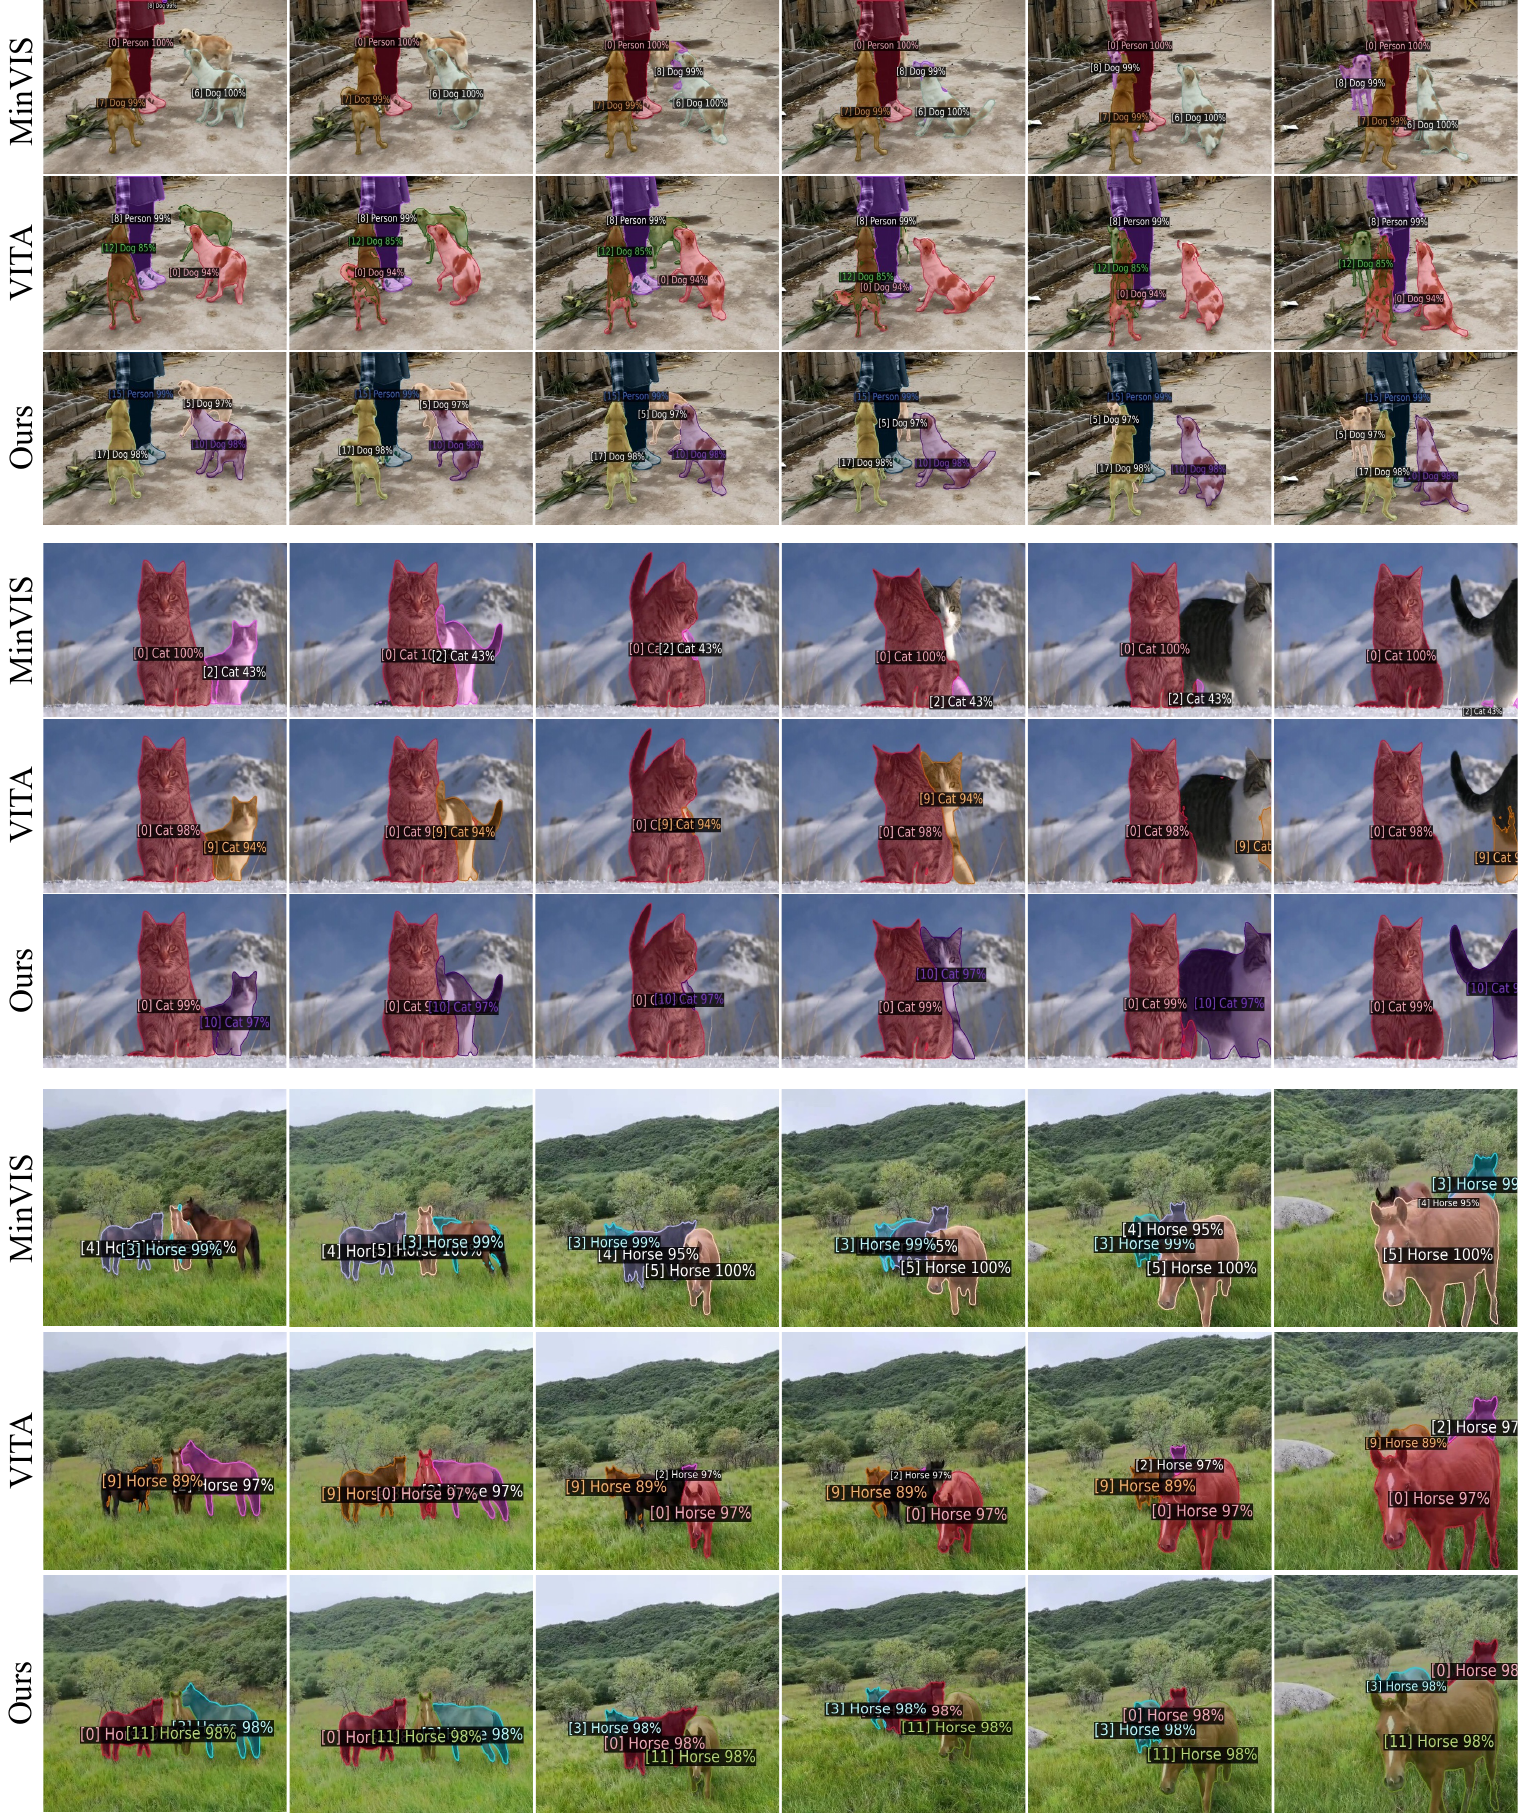}
\end{center}
\vspace{-3mm}
\caption{
Qualitative comparisons of our method, GenVIS, with the state-of-the-art methods: MinVIS~\cite{MinVIS} and VITA~\cite{VITA}.
% The videos on the left and right are from YouTube-VIS 2022~\cite{MaskTrackRCNN} and OVIS~\cite{OVIS-Dataset} datasets, respectively.
GenVIS shows impressive accuracy in these complicated scenes where the objects look similar crossing each other. Objects with the same identity are displayed in the same color.
}
%\vspace{-4mm}
\label{fig:qualitative_supp}
\end{figure*}

\paragraph{Dataset licenses} of COCO~\cite{COCO}, YouTube-VIS~\cite{MaskTrackRCNN}, and OVIS~\cite{OVIS-Dataset}: Attribution 4.0 International, CC BY 4.0, and CC BY-NC-SA 4.0, respectively.
